# Supplementary material for: Random Fourier Features for Operator-Valued Kernels
Source: arXiv:1605.02536 source file (2016-05-24)
Supplement: Supplementary file 1 [file commands.tex]

\newtheorem{theorem}{Theorem}[section]
\newtheorem{proposition}{Proposition}[section]
\newtheorem{corollary}{Corollary}[theorem]
\newtheorem{lemma}[theorem]{Lemma}
%\newtheorem{Definition}{Definition}[section]

\newenvironment{proof}[1][Proof]{\begin{trivlist}
\item[\hskip \labelsep {\bfseries #1}]}{\end{trivlist}}
\newenvironment{definition}[1][Definition]{\begin{trivlist}
\item[\hskip \labelsep {\bfseries #1}]}{\end{trivlist}}
\newenvironment{example}[1][Example]{\begin{trivlist}
\item[\hskip \labelsep {\bfseries #1}]}{\end{trivlist}}
\newenvironment{remark}[1][Remark]{\begin{trivlist}
\item[\hskip \labelsep {\bfseries #1}]}{\end{trivlist}}

\newcommand{\qed}{\nobreak \ifvmode \relax \else
      \ifdim\lastskip<1.5em \hskip-\lastskip
      \hskip1.5em plus0em minus0.5em \fi \nobreak
      \vrule height0.75em width0.5em depth0.25em\fi}

\DeclareMathOperator*{\argmin}{arg\,min}
\DeclareMathOperator*{\argmax}{arg\,max}
\DeclareMathOperator{\Tr}{Tr}
\DeclareMathOperator*{\sign}{sign}
\DeclareMathOperator{\lspan}{\overline{span}\;}
\DeclareMathOperator{\vect}{\bigoplus}
\DeclareMathOperator*{\Vect}{\bigoplus}
\newcommand{\ima}{\text{im}\;}
\newcommand{\Ima}{\text{Im}\;}
\newcommand{\Ker}{\text{Ker}\;}


% Florence's notations.
\def\expectation{{\mathbb{E}}}
\def\variance{{\mathbb{V}}}
\def\probability{{\mathbb{P}}}
%\def\covari{{\math{Cov}}

% Romain's notations.
% \def\expectation{{\bf\text{E}}}
% \def\variance{{\bf\text{Var}}}
% \def\probability{{\bf\text{Pr}}}

\def\param{\boldsymbol{\theta}}
\newcommand{\minimiser}{\hat\theta}
\newcommand{\parameter}{\theta}
\newcommand{\idim}{d}
\newcommand{\odim}{p}
\newcommand{\FT}[1]{\mathcal{F}\left[#1\right]}
\newcommand{\IFT}[1]{\mathcal{F}^{-1}\left[#1\right]}
\newcommand{\MGF}{\text{MGF}}

\DeclarePairedDelimiter\abs{\lvert}{\rvert}
\DeclarePairedDelimiter\norm{\lVert}{\rVert}
\DeclarePairedDelimiter\inner{\langle}{\rangle}
\DeclarePairedDelimiter\pairing{(}{)}
\DeclarePairedDelimiter\covariance{\text{Cov}_\mu[}{]}
\newcommand\dual[1]{\hat{#1}}
% \newcommand\dual[1]{#1}
\newcommand\conj[1]{\overline{#1}}

\makeatletter
\let\oldabs\abs
\def\abs{\@ifstar{\oldabs}{\oldabs*}}
%
\let\oldnorm\norm
\def\norm{\@ifstar{\oldnorm}{\oldnorm*}}
\makeatother

%% functions and operators
\def\density{\gamma}
\def\measure{\mu}
\def\adjoint{*}
\def\sech{\text{sech}}

%% Bold letter
\def\bfeps{\boldsymbol{\epsilon}}
\def\bfdelta{\boldsymbol{\delta}}
\def\bfDelta{\boldsymbol{\Delta}}
\def\bfa{{\mathbf a}}
\def\bfb{{\mathbf b}}
\def\bfc{{\mathbf c}}
\def\bft{{\mathbf t}}
\def\bfu{{\mathbf u}}
\def\bfv{{\mathbf v}}
\def\bfx{{\mathbf x}}
\def\bfy{{\mathbf y}}
\def\bfz{{\mathbf z}}
\def\bfB{{\mathbf B}}
\def\bfK{{\mathbf K}}
\def\bfX{{\mathbf X}}

%% Mathcalletter
\def\bmS{\mathcal{S}}
\def\bmB{\mathcal{B}}
\def\bmX{\mathcal{X}}
\def\bmY{\mathcal{Y}}
\def\bmC{\mathcal{C}}
\def\bmD{\mathcal{D}}
\def\bmL{\mathcal{L}}
\def\bmH{\mathcal{H}}
\def\bmF{\mathcal{F}}
\def\bmM{\mathcal{M}}
\def\bmN{\mathcal{N}}
\def\mRp{\mathbb{R}^p}
\def\mRd{\mathbb{R}^d}
